# Supplementary material for: Atomic clock transitions in silicon-based spin qubits
Source: arXiv:1301.6567 source file (2013-01-28)
Supplement: Supplementary file 1 [file SiBi-CT-SOM.pdf]

# Supplementary Material

## ESR- AND NMR-TYPE MAGNETIC FIELD "CLOCK" TRANSITIONS (CT)

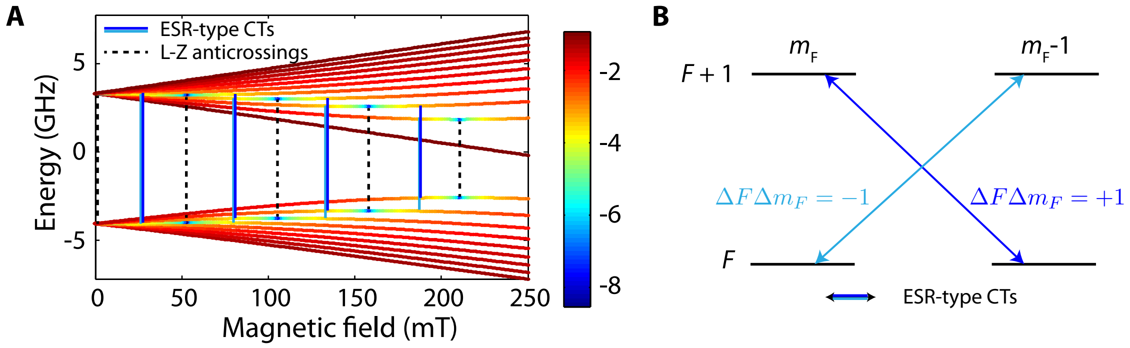


FIG. 1. **Description of ESR-type CTs. A,** The eigenstate energies of Si:Bi as function of magnetic field. The color scale shows the logarithmic distance to pure Bell states (Landau-Zener (L-Z) anticrossings) in the $|m_S, m_I\rangle$ basis, defined as $\log(|\theta - \pi/4|)$ for an eigenstate $|\Phi\rangle = \cos(\theta)\,|\mp\frac{1}{2}, m_I \pm \frac{1}{2}\rangle \pm \sin(\theta)\,|\pm\frac{1}{2}, m_I \mp \frac{1}{2}\rangle$. The Bell state at 0 mT is barely visible here due to degeneracy. **B,** ESR-type CTs with $\Delta F \Delta m_F = +1$ in dark blue and $-1$ in light blue. The four involved eigenstates, which are two pairs of hyperfine coupled states in the $|m_S, m_I\rangle$ basis, form a subspace of the Hilbert space.

Below we discuss the general requirements for ESR and NMR-type CTs for systems with electron spin $S = 1/2$ and nuclear spin $I$ and assuming an isotropic hyperfine coupling, with a particular focus on Group V donors in silicon. This letter is the first measurement of ESR-type CTs to our knowledge, though they have been theoretically described by Mohammady *et.al.* [1, 2] for donors in Si, in particular Bi. On the other hand, NMR-type CTs have been used in various systems in the past [3, 4], including in phosphorus donors in silicon [5], to reduce sensitivity to magnetic field inhomogeneities (i.e. increase frequency resolution) or to increase nuclear coherence times.

In the basis of the electron and nuclear spin $|m_S, m_I\rangle$, the isotropic hyperfine interaction $(A\vec{I} \cdot \vec{S})$ couples pairs of states within the Hilbert space such that $[\Delta m_S = \pm 1, \Delta m_I = \mp 1]$. In the strongly coupled electron-nuclear spin basis $|F, m_F\rangle$ $(F = I \pm S, m_F = m_S + m_I)$, these pairs of states share the same $m_F$ value. When the static magnetic field is increased, the Zeeman energy rises to the same order of magnitude as the hyperfine interaction, resulting

in avoided Landau-Zener crossings between states with $m_F \leq 0$ as shown in Figure 1A. ESR-type CTs are located between pairs of these avoided crossings.

At the intermediate fields relevant to CTs and Landau-Zener anticrossing, the eigenstates can be expressed either as being close to Bell states in the $|m_S, m_I\rangle$ basis, or still quite pure in the $|F, m_F\rangle$ basis. For example, the CT at 7.0317 GHz, explored in the main text, connects the following pairs of states:

$$-0.74\left|\frac{1}{2},-\frac{5}{2}\right\rangle + 0.67\left|-\frac{1}{2},-\frac{3}{2}\right\rangle \Leftrightarrow 0.74\left|\frac{1}{2},-\frac{3}{2}\right\rangle + 0.67\left|-\frac{1}{2},-\frac{1}{2}\right\rangle \quad \text{in the } |\mathrm{m_S},\mathrm{m_I}\rangle \text{ basis}$$

$$0.99\,|4,-2\rangle + 0.15\,|5,-2\rangle \Leftrightarrow -0.15\,|4,-1\rangle + 0.99\,|5,-1\rangle \quad \text{in the } |\mathrm{F},\mathrm{m_F}\rangle \text{ basis}$$

Hence, for convenience, we refer to these states by the dominant term in the $|F, m_F\rangle$ basis (i.e. $|4,-2\rangle$ and $|5,-1\rangle$ in the example above). The $\Delta F \Delta m_F = +1$ and $\Delta F \Delta m_F = -1$ CTs are each transitions between one state of the first Landau-Zener crossing to a second state of the second crossing, forming a 4-dimensional subspace of the Hilbert space (Figure 1B).

For non-integer [integer] values of $I$, there are $I + 1/2$ [$I$] Landau-Zener anticrossings and consequently $2(I - 1/2)$ [$2I$] ESR-type CTs. The minimum complexity required is thus a nuclear spin $I \geq 1$ to have at least two pairs of hyperfine coupled states, which is not the case for phosphorus donors ($^{31}$P has $I = 1/2$).

Arsenic ($^{75}$As, $I = 3/2$) and antimony ($^{121}$Sb, $I = 5/2$ and $^{123}$Sb, $I = 7/2$) have sufficient nuclear spin to permit ESR-type CTs, however the hyperfine coupling is relatively weak ($A \sim$ 198, 186 and 101 MHz, respectively), so the avoided crossings are found at low magnetic field and transition frequencies (see Table I). Bismuth $^{209}$Bi with $I = 9/2$ and $A = 1.475$ GHz is thus the optimal Group V donor in silicon from the point of view of CTs, possessing four of them at GHz frequencies.

| | $^{75}$As ($I = 3/2$) | $^{121}$Sb ($I = 5/2$) | | $^{123}$Sb ($I = 7/2$) | | | $^{209}$Bi ($I = 9/2$) | | | |
|---|---|---|---|---|---|---|---|---|---|---|
| $\Delta F = +1, m_F =$ | $-1 \leftrightarrow 0$ | $-1 \leftrightarrow 0$ | $-2 \leftrightarrow -1$ | $-1 \leftrightarrow 0$ | $-2 \leftrightarrow -1$ | $-3 \leftrightarrow -2$ | $-1 \leftrightarrow 0$ | $-2 \leftrightarrow -1$ | $-3 \leftrightarrow -2$ | $-4 \leftrightarrow -3$ |
| Magnetic field (mT) | 3.8 | 3.4 | 10.4 | 1.8 | 5.5 | 9.3 | 26.6 | 79.8 | 133.3 | 187.8 |
| Frequency (GHz) | 0.384 | 0.552 | 0.482 | 0.403 | 0.376 | 0.314 | 7.338 | 7.032 | 6.372 | 5.214 |

TABLE I. **Summary of ESR-type magnetic-field CTs in donors in silicon.** CTs exist in pairs ($\Delta F \Delta m_F = \pm 1$) separated by less than 0.15 mT in magnetic field and 3 MHz in frequency. Phosphorus does not possess any CT due to its small nuclear spin ($I = 1/2$).

As $df/dB \to 0$, the next figure of merit is the electron transition probability amplitude,

which is always 50% of the high field limit for ESR-types. This means that manipulation times are only slightly reduced while electron coherence times $T_{2\mathrm{e}}$ are drastically increased. Conversely, as flip-flops between two donor electron spins follow the square of this probability amplitude, the flip-flopping rate remains strong, limiting $T_{2\mathrm{e}}$ as observed and explained in the main text.

NMR-type CTs occur at strong magnetic field (in Si:Bi, 0.3 T $< B_0 <$ 5 T, from $m_I = -9/2$ at low field to $m_I = 9/2$ at high field) and as such are transitions between quasi-pure states in the $(m_S, m_I)$ basis. NMR-type CTs possess a change in nuclear spin state of $\Delta m_I = 1$ and can be manipulated in a conventional electron nuclear double resonance (ENDOR) or NMR experiment. Amongst the NMR-type CTs, those at higher magnetic fields have a smaller electron spin component. This leads to a reduced coupling to the environment, but also increased spin manipulation times, converging to that of a regular NMR transition (typically $\sim 10$ $\mu$s).

## ESR LINEWIDTHS

Measurements of spin linewidths provide important details regarding the spin environment, yielding information on crystalline defects and strains amongst other properties. Line broadening arises from a variation in either the hyperfine interaction ($\Delta A$) or the magnetic field ($\Delta B$) (or g-tensor) across the sample. They can either be measured in a magnetic field-swept spectrum where (to first order):

$$\Delta B_{Total} = \Delta B + \frac{dB}{df}\frac{df}{dA}\Delta A \tag{1}$$

or in Fourier-Transform (FT) ESR where the FT of the free induction decay after a $\pi/2$ rotation gives the spectrum in the frequency domain. In this case, (to first order):

$$\Delta f = \frac{df}{dB}\Delta B + \frac{df}{dA}\Delta A \tag{2}$$

At the CT where $dB/df \to \infty$, the linewidth in the magnetic field domain broadens strongly until it becomes limited by the second order dependence on magnetic field. Both $\Delta B$ and $\Delta A$ can be identified by varying the transition frequency and fitting numerically knowing $\frac{dB}{df}\frac{df}{dA}$. To confirm that this change in linewidth is strictly related to the term $df/dB$, we can make use of the FT ESR technique which simplifies at the CT to $\Delta f = \frac{df}{dA}\Delta A$, where

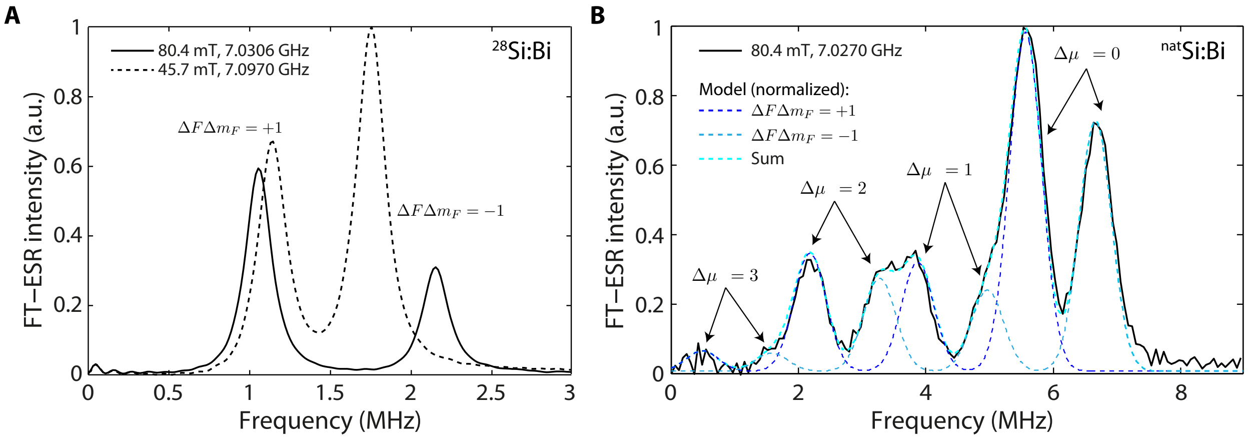


FIG. 2. **FT-ESR around the CT.** Each spectrum is the FT of the free induction decay taken using a microwave frequency slightly below resonance (values given in legend). **A,** For the case of $^{28}$Si:Bi, we observe two peaks in the ESR spectrum around the CT, corresponding to the transitions $\Delta F \Delta m_F = \pm 1$. Spectra are shown as measured at two settings of magnetic field/microwave frequency. In the magnetic field domain, the ESR linewidths in these two cases are 1.6 mT close to the CT and 0.07 mT farther away (see Figure 1 of the main manuscript), however in the frequency domain as shown above, the ESR linewidths are constant. **B,** In $^{nat}$Si:Bi, these two primary ESR transitions are further split into sub-peaks, corresponding to a mass-effect from nearest neighbour Si atoms. Each shift of one neutron mass ($\Delta\mu$) yields a shift of $-1.7$ MHz in transition frequency (or 0.024% change in the hyperfine coupling A). Dashed lines show simulated peaks whose intensity is calculated from a trinomial distribution of $^{30}$Si, $^{29}$Si and $^{28}$Si isotopes in $^{nat}$Si (with respective concentration 3.1%, 4.7% and 92%). As the FT-ESR is derived from the free induction decay, the intensities are normalized by the FT of the inhomogeneous decay $T_{2e}{}^*$ (Lorentzian) and the cavity bandwidth.

$df/dA$ is quasi-constant around the CT. In Figure 2A, the linewidth is indeed constant about 270 kHz.

In natural silicon, the elimination of the $\Delta B$ term dramatically reduces the ESR linewidth. Away form the CT (e.g. at X-band), $\Delta B$ is normally around 4 G due to unresolved coupling to $^{29}$Si nuclear spins. In the frequency domain, this would be equivalent to nearly 12 MHz, hiding multiple spectral features. First, the two transitions $\Delta F \Delta m_F = \pm 1$ would not be resolvable. Second, as show in Figure 2B, we observe several other peaks (absent in isotopically pure $^{28}$Si samples) which arise from variations in the hyperfine coupling

due to the total mass of nearest-neighbour silicon atoms ($^{28}$Si, $^{29}$Si and $^{30}$Si). This effect is described in full detail, including ENDOR experiments, in a forthcoming work [6].

## ELECTRIC FIELD CLOCK TRANSITIONS

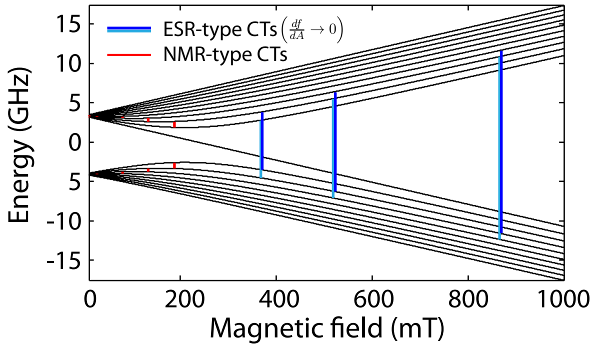


FIG. 3. **Clock transitions in Si:Bi where $df/dA = 0$ which should be robust to electric field noise.** Both ESR- and NMR-type CTs can be observed, as for magnetic-field CTs. One further ESR-CT is found at higher magnetic fields (2.6 T, not shown).

In the experiments reported in the main text, CTs were used to reduce the sensitivity of electron spin to magnetic field variations, as quantified by $df/dB$. While magnetic field noise is indeed the main decoherence mechanism in bulk materials, this may not be the case in nanoscale devices where the electric field at interfaces could couple strongly with both the donor electron and nuclear spins through the hyperfine interaction (and also, to lesser extent, through a modulation in the electron spin g-factor). The sensitivity of a spin to this effect can be quantified by the gradient of the frequency with respect to the hyperfine constant $df/dA$, combined with values for the DC Stark effect for donors in silicon (which for Group V donors is in the order of $10^{-3}$ $\mu$m$^2$/V$^2$, as a fractional change in the hyperfine coupling [7, 8]). Those CTs which will be most robust to electric field noise ($df/dA \to 0$) are identified in Si:Bi in Figure 3 and in Table II for all Group V donors in silicon.

In practice, both magnetic and electric field fluctuations will participate to the donor spin decoherence. There will thus be an optimal CT, at a specific magnetic field and frequency, where the coherence time would be maximum. For example, the magnetic field CT near 188 mT in Bi has the lowest value of $df/dA$ out of the four possible CTs. In other scenarios, it might be advantageous to minimise the inhomogeneous broadening as much as possible

| | $^{75}$As ($I=3/2$) | $^{121}$Sb ($I=5/2$) | | $^{123}$Sb ($I=7/2$) | | | $^{209}$Bi ($I=9/2$) | | | |
|---|---|---|---|---|---|---|---|---|---|---|
| $\Delta m_S=+1, m_I=$ | $-1/2$ | $-1/2$ | $-3/2$ | $-1/2$ | $-3/2$ | $-5/2$ | $-1/2$ | $-3/2$ | $-5/2$ | $-7/2$ |
| Magnetic field (mT) | 53 | 117 | 39 | 114 | 38 | 23 | 2607 | 868 | 519 | 369 |
| Frequency (GHz) | 1.43 | 3.21 | 0.92 | 3.17 | 0.98 | 0.49 | 72.64 | 23.18 | 12.57 | 7.30 |

TABLE II. **Summary of ESR-type electric-field CTs in donors in silicon.** At the given magnetic fields, the electron and nuclear spins are weakly coupled and the eigenstates must thus be expressed in the $|m_S, m_I\rangle$ basis. The $[\Delta m_S=\pm1, \Delta m_I=\mp2]$ ($\Delta F\Delta m_F=-1$) transitions are nearly completely forbidden here; they would have been found at the same magnetic field as the $[\Delta m_S=\pm1, \Delta m_I=0]$ ($\Delta F\Delta m_F=+1$) transitions, but separated by less than 40 MHz in frequency.

(e.g. for coupling a spin ensemble to a microwave resonator), and this would also require different optimal operating points within the Hilbert space of the bismuth electron and nuclear spins.

---


[1] M. Mohammady, G. W. Morley, and T. S. Monteiro, Phys. Rev. Lett. **105**, 067602 (2010).

[2] M. H. Mohammady, G. W. Morley, A. Nazir, and T. S. Monteiro, Phys. Rev. B **85**, 094404 (2012).

[3] W. Hardy, A. Berlinsky, and L. Whitehead, Physical Review Letters **42**, 1042 (1979).

[4] J. Longdell, A. Alexander, and M. Sellars, Physical Review B **74**, 195101 (2006).

[5] M. Steger *et al.*, Journal of Applied Physics **109**, 102411 (2011).

[6] A. Tyryshkin *et al.*, in preparation (2013).

[7] F. Bradbury *et al.*, Physical Review Letters **97**, 176404 (2006).

[8] R. Rahman *et al.*, Physical Review Letters **99**, 36403 (2007).
